# Supplementary material for: Analyzing and Improving Neural Networks by Generating Semantic Counterexamples through Differentiable Rendering
Source: arXiv:1910.00727 source file (2020-07-17)
Supplement: Supplementary file 1 [file Appendix.tex]

\section{Constructions}

Recall that $\bfz=(x,y)$ where $x = \render(\seminp)$ and $y=F(x)=F(\render(\seminp))$.
Consider the loss function $\ell_F(x,y)$. Let $\seminp_0$ be a starting semantic feature vector that we wish to perturb
into a semantic counterexample.
The derivative with respect to $\seminp$, evaluated at $\seminp_0$ is $\left.\left[\frac{\partial\render}{\partial\seminp}\right]^{\top}\right\vert_{\seminp_0}\left.\nabla_{\bfz} \ell_F (\bfz)\right\vert_{\bfz = (\render(\seminp_0), F(\render(\seminp_0)))}$ (the notation $\left.\left[\frac{\partial\render}{\partial\seminp}\right]^{\top}\right\vert_{\seminp_0}$ is the transposed Jacobian matrix of $\render$ as a vector-valued function of $\seminp$, evaluated at $\seminp_0$, and  $\nabla_{\bfz} L_F(\bfz) |_{\bfz = (\render(\seminp_0), F(\render(\seminp_0)))}$ is the derivative evaluated at 
$(\render(\seminp_0), F(\render(\seminp_0)))$.

The semantic version of FGSM ({\it sFGSM}) will produce the following $\semce$:
\begin{equation}
\label{eq:sFGSM}
\semce  = \seminp_0 \varepsilon \signf\left(
\left.\left[\tfrac{\partial\render}{\partial\seminp}\right]^{\top}\right\vert_{\seminp_0}\left.\nabla_{\bfz} \ell_F (\bfz)\right\vert_{\bfz = (\render(\seminp_0), F(\render(\seminp_0)))}
%}
%
%\left.\left[\tfrac{\partial\re}{\partial\theta}\right]^{\top}\right\vert_{(x, \perp)}\left.\nabla_{\bfz} L_F (\bfz) \right|_{\bfz = \tau(x, \perp)}
%
\right)
\end{equation}

% \begin{equation}
% \label{eq:sFGSM}
% \bftheta^\star  = \varepsilon \signf(\nabla_{\bfz} L_F (\bfz) |_{\bfz = x} \nabla_{\theta} \tau(x,\theta)) |_{\theta = \perp}
% \end{equation}

The adversarial example $A(x)$ is $\tau(x,\bftheta^\star)$. Note that we do not assume any special properties about $\tau$, such as  linearity. We only assume that $\tau$ is differentiable. %, which get because of the user of differentiable rendering. 

%\sanjit{Modify the material below in a manner similar to FGSM above}

In a similar manner a semantic version of the PGD attack ({\it sPGD}) can be constructed.  Let $\bftheta_0$ 
be the semantic feature vector we wish to perturb. The update step corresponds to the following equation:
\begin{equation}
\label{eq:PGD}
\theta_{k+1}  = \Pi_{ B_\mu (\theta_0 , \epsilon)} \left( \theta_k \oplus \seminp_0 \varepsilon \signf\left(
\left.\left[\tfrac{\partial\render}{\partial\seminp}\right]^{\top}\right\vert_{\seminp_k}\left.\nabla_{\bfz} \ell_F (\bfz)\right\vert_{\bfz = (\render(\seminp_k), F(\render(\seminp_k)))}
\right)

\end{equation}

% \begin{eqnarray*}
%   \bftheta_{k+1}  & = & \Pi_{B_\mu (\bftheta_0,\varepsilon)}
%   (\bftheta_k \; \oplus \;
%   \varepsilon \signf(\nabla_{\bfz} L_F (\bfz) |_{\bfz = x} \nabla_{\theta} \tau(x_k,\theta) |_{\theta = \bftheta_k}) ) \\
%   x_{k+1} & = & \tau (x_0,\bftheta_k)
% \end{eqnarray*}
Note that $\Pi_{B_\mu (\cdot,\cdot)}$ is the projection operator in the parameter space $\Theta$. We also assume that the 
projection operator will keep the parameters in the feasible 
set, which depends on the image (\eg translation does not take the 
car off the road). 

Even though we only considered semantic versions of FGSM, Carlini-Wagner, and PGD, our technique can be used to transform any attack algorithm.
% such as Carlini \& Wagner~\cite{carlini2017towards} 
% that adds a perturbation $\delta$, to its ``semantic version''. 

\section{Implementation} 
\label{sec:implementation}

\subsection{Semantic Features}
\label{semantic}

Recall that we generate augmenting samples by strategically perturbing semantic features. In the case of VKITTI (using 3D-SDN), the semantic features include (a) \cars: the car's texture codes which change its color, (b) \sky: the weather and time of day, (c) \foliage: the surrounding foliage and scenery, (d) \rotate: the car's orientation, (e) \translate: the car's position in 2D, and (f) \FFD: the 3D mesh which provides structure to the car. In the case of ShapeNet (using Redner), the semantic features include: (a) \pose:, (b) \vertex:, and (c) \lighting: \varun{missing description of each of the semantic parameters for redner; add a note on "units" for each of these hyperparameters}

\subsection{Attacks}
\label{attacks}

Before we discuss specifics about the strategies we use to generate augmenting samples, we need to understand how the semantic parameter space can be manipulated. In particular, we wish to answer the question: {\em Which semantic parameters do we change?} In the pixel perturbation setting, all pixels are equal \ie any pixel can be perturbed. Whether such uniformity naturally exists in the semantic space is unclear. However, we have additional flexibility; for each rendering framework, we can choose to modify any of the above listed semantic parameters independently without altering the others, \ie perform {\em single parameter modifications}. Alternatively, we can modify any subset of the parameters in unison, \ie perform {\em multi-parameter modifications}. 

\noindent{\bf 1. Redner:} We utilize 3 candidate algorithms to induce meaningful semantic modifications: sPGD, sFGSM, and sCW. Our experiments show that varying the \lighting semantic parameter does not result in information gain, and we do not discuss it in the remainder of the paper. We report the best values after an extensive hyperparameter sweep. 
\begin{itemize}
\itemsep0em
\item For sPGD, the scaling factor $\alpha$ is set to $0.5$ for \pose, and $5.0$ for \vertex. %wait what? @varun thats the epsilon bounds. not the learning rate.
\item For sCW, the attack was formulated according to \cite{carlini2017towards} with the 2-norm used for our distance metric. The attack was untargeted, as we sought just to induce a misclassification of some kind while minimizing the 2-norm of the distance between the old semantic feature vector and the new one. The learning rate used was $0.30$ for \pose and $0.01$ for \vertex
% \varun{@lakshya: add some notes on how the attack is formulated i.e. what is penalized. from our discussion, you said that for each semantic parameter, the 2-norm of the difference between the new rendered output and the original rendered output was minimized?}
\item For sFGSM, the step-size hyperparameter $\varepsilon$ is set to $0.15$ for \pose, and $0.002$ for \vertex.
\end{itemize}

\noindent{\bf 2. 3D-SDN:} We utilize an iterative variant of FGSM to modify the semantic parameters (henceforth referred to as sFGSM$_\text{3D-SDN}$). Recall that in FGSM, the degree of modification of the input is determined by the steps-size hyperparameter $\varepsilon \in [0,1]$. In the context of generating augmenting samples, the value of $\varepsilon$ is proportional to the magnitude of the geometric and textural changes induced; the effect depends on the semantic parameter under consideration. Large values of $\varepsilon$ result in unrealistic images rendered. To avoid such issues and to simulate {\em realistic} transformations, we use a different step-size for each semantic parameter. We report the results of our hyperparameter sweep: (a) \cars: $\varepsilon$ = 0.05, (b) \sky: $\varepsilon$ = 0.25, (c) \foliage: $\varepsilon$ = 0.10, (d) \rotate: $\varepsilon$ = 0.01, (e) \translate: $\varepsilon$ = 0.01, and (f) \FFD: $\varepsilon$ = 0.025. 

We stress that for both differentiable graphics frameworks, these hyperparameters were obtained after extensive visual inspection (by 3 viewers independently); in \S~\ref{realism}, we validate the realism of the generated samples. An added benefit of our particular choice of hyperparameters (for 3D-SDN) is that it enables us to use the same ground truth labels throughout our experiments; the produced SAEs have bounding box coordinates that enable us to use the same ground truth labels as their benign counterparts\footnote{This fact is useful when we evaluate model robustness through retraining the models with SAEs as inputs, which we discuss in \S~\ref{augmentation}}. 
